# Supplementary material for: Neural Control Variates with Automatic Integration
Source: arXiv:2409.15394 source file (2024-09-23)
Supplement: Supplementary file 1 [file supp.tex]

\section{Differential Spatial Integration}
\paragraph{Integration on a 2D Circle.}  Here we consider $\Omega$ contain points on the 2D circle centered at $c\in\Re^2$ with radius $R>0$: $\{p\in \Re^2| \|p - c\| <= R\}$. In this case, the parameterization of the domain can be defined as:
\begin{align}
    C(\theta) = R[\sin(\theta), \cos(\theta)]^T, \theta \in [0, 2\pi].
\end{align}
The integration over the circle can be expressed as the following line integral:
\begin{align}
    \int_{x\in \Omega} f(x)dx = R\int_{0}^{2\pi} f(C(\theta))d\theta
\end{align}

\paragraph{Integrating inside a 2D Circle.} Here we consider $\Omega$ is a 2D circle centered at $c\in \Re^2$ with radius $R>0$: $\{p\in \Re^2| \|p - c\| <= R\}$
then it can be parameterized by the following function:
\begin{align}
    B(r, \theta) = r[\sin(\theta), \cos(\theta)]^T, \quad r \in [0, R], \theta \in [0, 2\pi].
\end{align}
This parameterization gives us integration on the circle using polar coordinates:
\begin{align}
    \int_{x\in\Omega} f(x)dA = \int_{0}^R\int_{0}^{2\pi}r\cdot f(B(r,\theta))\ d\theta dr.
\end{align}
This integration shows up in applications including Walk-on-sphere Monte Carlo solvers for Poisson equations.

\paragraph{Integration on a 3D sphere.} Here we consider $\Omega$ to be the surface of a 3D sphere centered at $\vec{c}\in\Re^d$ with radius $R > 0$: $\Omega=\{\vec{p}\in\Re^3 | \|\vec{p}-\vec{c}\|=R\}$. The sphere can be parameterized by the spherical coordinates:
\begin{align}
S_R(\theta, \phi) = R[\sin(\theta)\cos(\phi), \sin(\theta)\sin(\phi), \cos(\theta)]^T, \theta \in [0, \pi], \phi \in [0, 2\pi].
\end{align}
The spatial integration can be written as :
\begin{align}
\int_{x\in\Omega}f(x)dS = R^2\int_{0}^{\pi}\int_0^{2\pi} \sin(\theta) f(S_R(\theta, \phi))d\phi d\theta
\end{align}
This integration is useful in Walk-on-sphere Monte Carlo solvers for 3D shapes as well as solving light transport equations for physics-based rendering.

\paragraph{Integration inside a 3D Sphere.}  Let $\Omega$ be all the points on a 3D sphere centered at $\vec{c}\in\Re^d$ with radius $R>0$: $\Omega=\{\vec{p}\in\Re^3 | \|\vec{p} - \vec{c}\| \leq R\}$. We can use spherical coordinates to parameterize this domain:
\begin{align}
    S(r, \theta, \phi) = r[\sin(\theta)\cos(\phi), \sin(\theta)\sin(\phi), \cos(\theta)]^T, r > 0, \theta \in [0, \pi], \phi \in [0, 2\pi].
\end{align}
The integration can be written as the following:
\begin{align}
    \int_{x\in\Omega}f(x)dA = \int_{0}^R\int_{0}^{\pi}\int_0^{2\pi} r^2\sin(\theta) f(S_R(\theta, \phi))d\phi d\theta dr
\end{align}
This integration shows up in Walk-on-sphere algorithms in solving variable coefficient elliptic equations.
